# Supplementary material for: Automated simulations beyond the Standard Model: supersymmetry
Source: arXiv:1907.04898 ancillary file (2019-07-10)

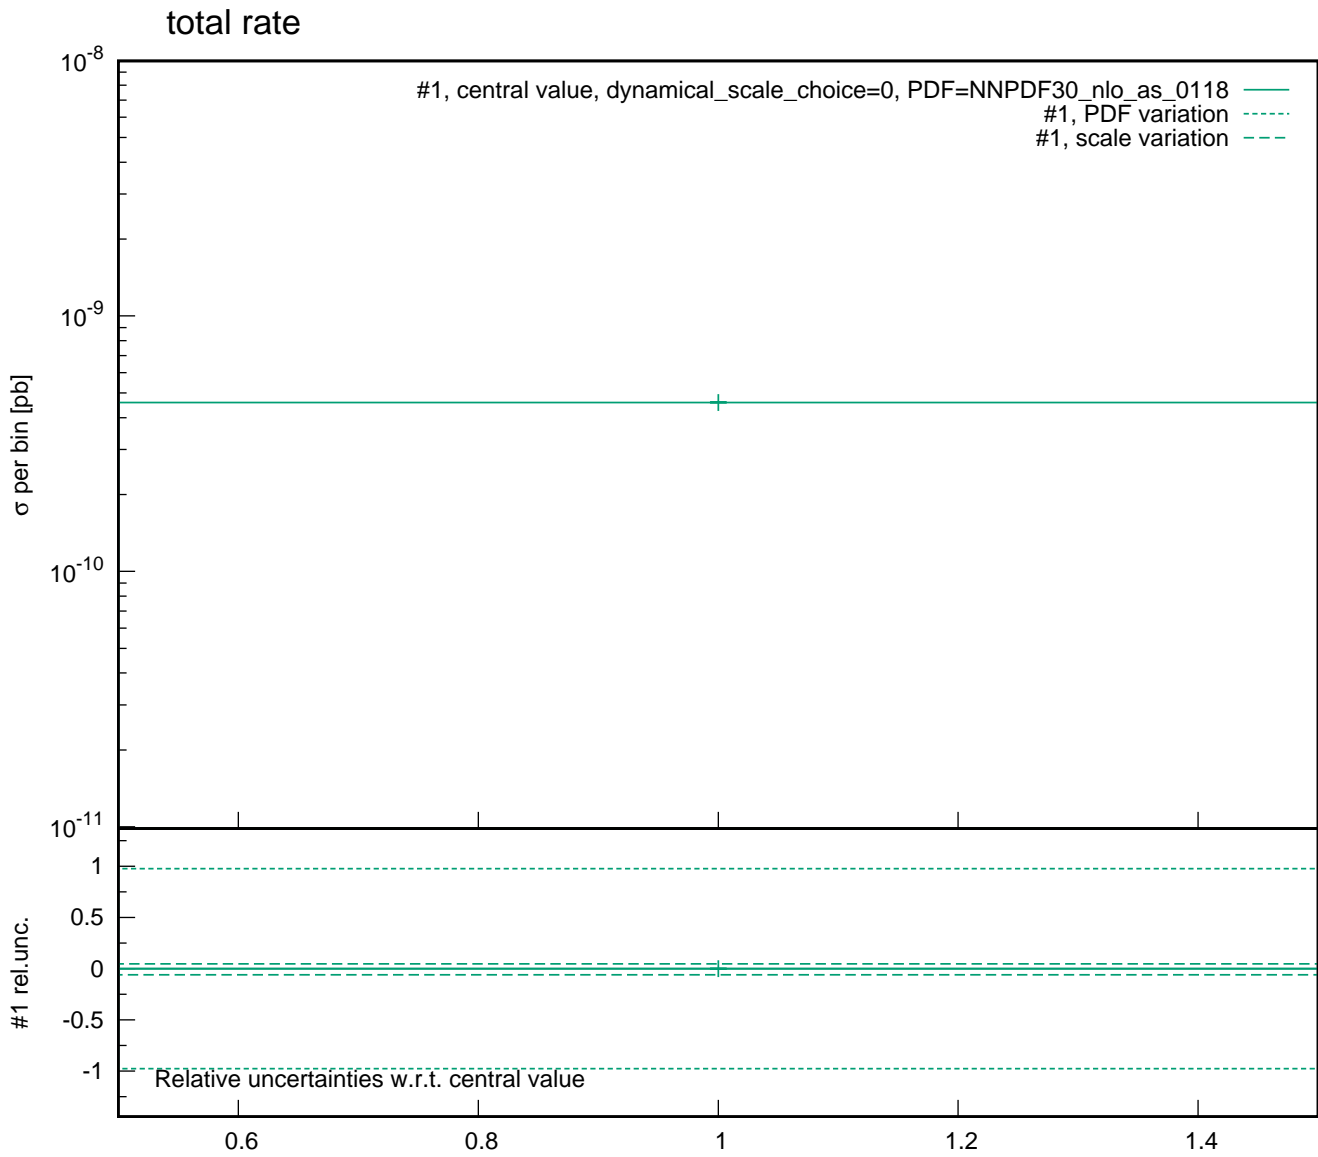

# total rate Born

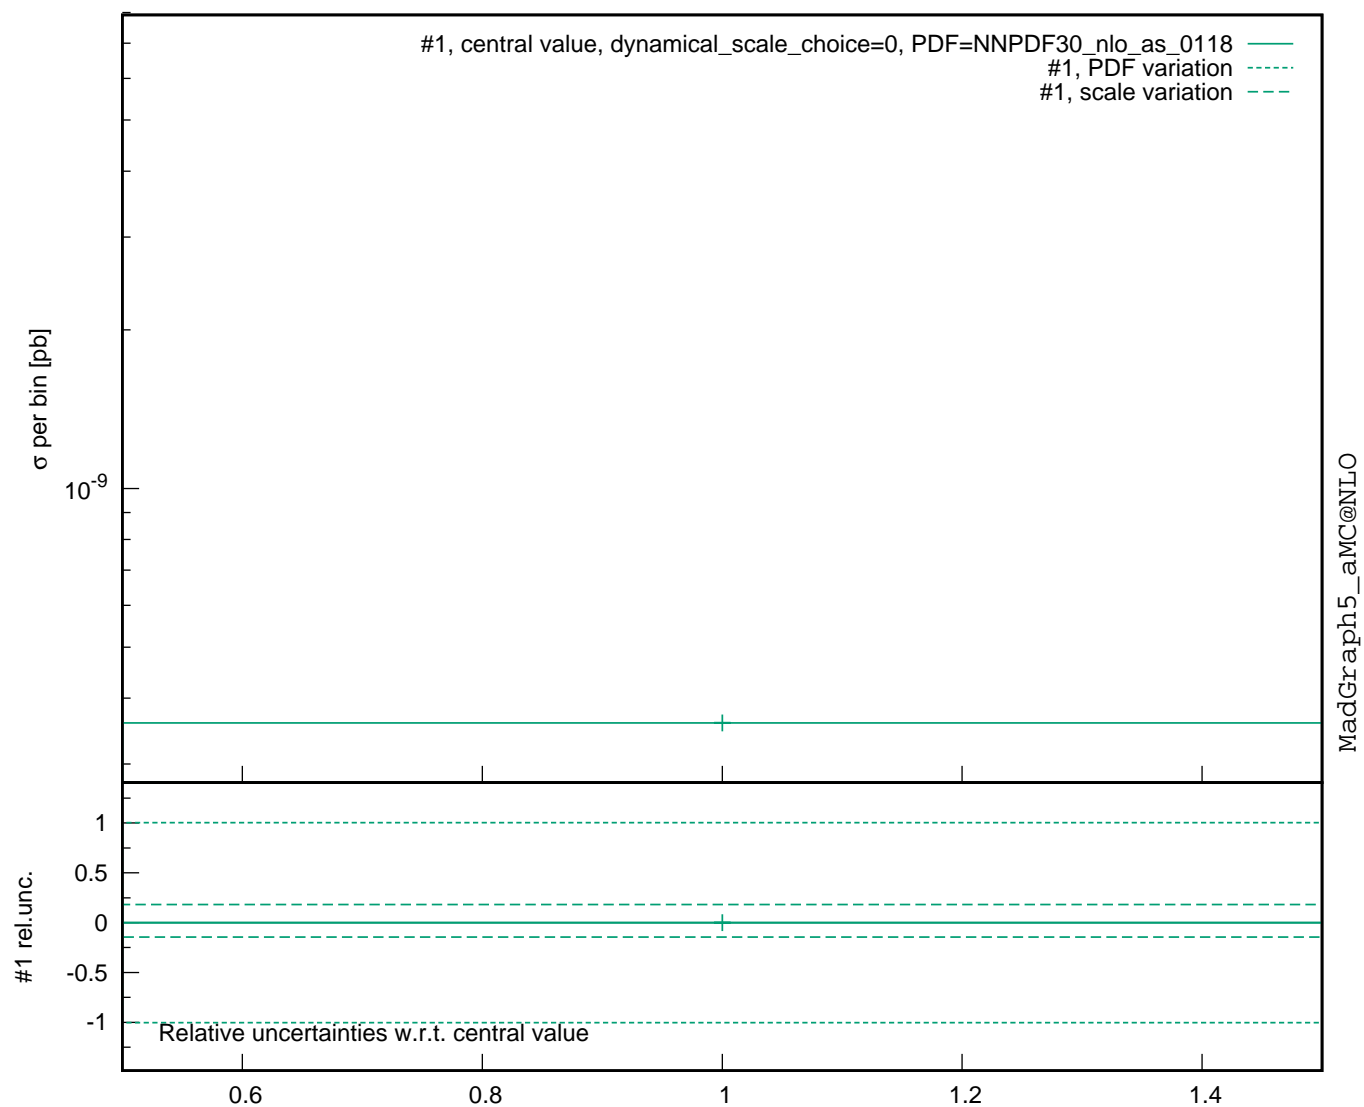

Supplement: Supplementary file 11 [file MADatNLO.pdf]
